# Supplementary material for: Reversal of Solvent Migration in Poroelastic Folds
Source: arXiv:2209.00887 ancillary file (2022-09-02)
Supplement: Supplementary file 1 [file supplement.pdf]

# Supplementary Information: Reversal of Solvent Migration in Poroelastic Folds


Mees M. Flapper,[1] Anupam Pandey,[2] Stefan Karpitschka,[3] and Jacco H. Snoeijer[1]

[1] *Physics of Fluids Group, Faculty of Science and Technology, Mesa+ Institute, University of Twente, 7500 AE Enschede, The Netherlands*

[2] *Department of Mechanical & Aerospace Engineering and BioInspired Institute, Syracuse University, Syracuse, NY 13244, USA*

[3] *Max Planck Institute for Dynamics and Self-Organization, 37077 Göttingen, Germany*



(Dated: September 1, 2022)


## I. THE FINGER TENSOR IN A FOLD

We here present details on how the Finger tensor is computed from the fold mapping:

$$\varphi = b\Phi, \quad r/\lambda(r) = R, \tag{1}$$

The Finger tensor is defined as $\mathbf{B} = \mathbf{F}\cdot\mathbf{F}^T$, where $\mathbf{F}$ is the gradient deformation tensor. In polar coordinates, this takes the form [1]

$$\mathbf{F} = \begin{pmatrix} \frac{\partial r}{\partial R} & \frac{1}{R}\frac{\partial r}{\partial \Phi} \\ r\frac{\partial \varphi}{\partial R} & \frac{r}{R}\frac{\partial \varphi}{\partial \Phi} \end{pmatrix} = \begin{pmatrix} \frac{\lambda}{1-r\lambda'/\lambda} & 0 \\ 0 & b\lambda \end{pmatrix} \quad \Rightarrow \quad \mathbf{B} = \begin{pmatrix} \left(\frac{\lambda}{1-r\lambda'/\lambda}\right)^2 & 0 \\ 0 & (b\lambda)^2 \end{pmatrix}. \tag{2}$$

In the main text we further used that $|r\lambda'/\lambda| \ll 1$ as one approaches the tip ($r\to 0$), which simplifies the analysis. This property follows from the fact that (i) the mapping should remain invertible, and (ii) exhibit a finite elastic energy. For the mapping to remain invertible, as is necessary in elasticity, we must impose that $J = \det(\mathbf{F})$ be finite everywhere. This includes the tip, where we have $J \to J_0 > 0$. This gives a condition

$$\frac{b\lambda^2}{1 - r\lambda'/\lambda} \simeq J_0, \tag{3}$$

for small $r$. To identify the asymptotics, we solve this first order ODE for $\lambda(r)$, taking $J_0$ constant, which gives

$$\lambda(r) = \frac{\sqrt{J_0/b}}{\left(1+(a/r)^2\right)^{1/2}}, \tag{4}$$

where $a$ is an integration constant. We separately consider $a = 0$ and $a \neq 0$. In the latter case, we find for $r \ll a$ that $\lambda \sim r$. In terms of the radial stretch, this implies $\partial r/\partial R \sim 1/r$ which generates an elastic energy density $W \sim 1/r^2$ (or worse, if we go beyond neo-Hookean networks). This energy is non-integrable in a corner, since the total energy $\int dA\, W \sim \int dr\, rW \sim \ln r \to \infty$. Hence, the solution $\lambda(r)$ with $a \neq 0$ comes with an infinite energy and thus must be excluded. We are left with imposing $a = 0$, which gives to leading order that $\lambda$ approaches a constant value $\lambda \simeq \sqrt{J_0/b}$. The solutions $\lambda(r)$ that are identified in the manuscript each have algebraic approach to this constant, i.e. $\lambda - \sqrt{J_0/b} \sim r^\alpha$ with $\alpha > 0$. Such corrections indeed have $r\lambda'/\lambda \sim r^\alpha \to 0$, as was used in the main text.

## II. STRAIN STIFFENING

We provide the technical steps leading to $\phi(r)$ presented in the main text for models that exhibit strain stiffening. Such models exhibit an elastic stress $\boldsymbol{\sigma}_{\mathrm{el}} = \psi(I)G\mathbf{B}$. For the Arruda-Boyce (AB) model, the strain-stiffening function takes the form [2, 3]

$$\psi_{AB}(I) = \frac{\beta(\hat{\lambda}_r)}{3\hat{\lambda}_r}, \tag{5}$$

where $\hat{\lambda}_r$ is the "mean relative chain stretch", measured with respect to its maximum extension. In terms of the first invariant, it is thus defined as $\hat{\lambda}_r = \sqrt{I/I_{\rm max}}$. The function $\beta(\lambda)$ is defined via the inverse Langevin function, as

$$\hat{\lambda}_r = \coth(\beta) - \frac{1}{\beta}. \tag{6}$$

For small $\beta$, one finds $\hat{\lambda}_r = \beta/3$, such that $\psi_{AB} \to 1$. However, the function $\beta$ diverges as $\hat{\lambda}_r \to 1$, which can be seen upon the large $\beta$ expansion:

$$\hat{\lambda}_r = \frac{e^{2\beta}+1}{e^{2\beta}-1} - \frac{1}{\beta} = \frac{1+e^{-2\beta}}{1-e^{-2\beta}} - \frac{1}{\beta} \simeq 1 - \frac{1}{\beta}, \tag{7}$$

so that

$$\beta \simeq \frac{1}{1-\hat{\lambda}_r} = \frac{1}{1-\sqrt{I/I_{\rm max}}}, \quad \Rightarrow \quad \psi_{AB} \simeq \frac{1}{3(1-\sqrt{I/I_{\rm max}})}. \tag{8}$$

For the Gent (G) model in plain strain, the strain-stiffening function is defined by [3, 4]

$$\psi_G = \frac{I_{\rm max}-2}{I_{\rm max}-I}, \tag{9}$$

which close to $I_{\rm max}$ gives the expansion

$$\psi_G \simeq \frac{1}{1-I/I_{\rm max}}. \tag{10}$$

While the expansions for $\psi_{AB}$ and $\psi_G$ are slightly different, both models produce the same asymptotics for $\phi(r)$ as described in the main text. Specifically, we found a divergence as $\psi \sim 1/r^{1-b^2}$, in the fold with $b<1$, such that for either the Arruda-Boyce or Gent models, we find to leading order in small $r$

$$I/I_{\rm max} = 1 - k\, r^{1-b^2}. \tag{11}$$

Only the numerical constant $k>0$ differs between the two models. Next, evaluating $I = {\rm tr}(\mathbf{B})$ and $J = \det(\mathbf{B})^{1/2}$ directly from the Finger tensor, one finds $J = I/(b^{-1}+b)$, such that

$$J \simeq \frac{I_{\rm max}(1-k\, r^{1-b^2})}{b^{-1}+b}, \quad \Rightarrow \quad \phi = 1 - 1/J \simeq 1 - \frac{b^{-1}+b}{I_{\rm max}}\left[1 + k\, r^{1-b^2}\right]. \tag{12}$$

This is the result given in the main text.


[1] M. Singh and A. C. Pipkin, Note on ericksen's problem, Zeitschrift für angewandte Mathematik und Physik ZAMP **16**, 706 (1965).

[2] E. M. Arruda and M. C. Boyce, A three-dimensional constitutive model for the large stretch behavior of rubber elastic materials, Journal of the Mechanics and Physics of Solids **41**, 389 (1993).

[3] C. O. Horgan, The remarkable gent constitutive model for hyperelastic materials, International Journal of Non-Linear Mechanics **68**, 9 (2015).

[4] A. N. Gent, A new constitutive relation for rubber, Rubber Chemistry and Technology **69**, 59 (1996).
